# Supplementary material for: Multi-agent Long-term 3D Human Pose Forecasting via Interaction-aware Trajectory Conditioning
Source: arXiv:2404.05218 source file (2024-04-08)
Supplement: Supplementary file 1 [file X_suppl.tex]

\clearpage
\setcounter{page}{1}
\maketitlesupplementary

\begin{figure*}[t]
\includegraphics[width=\textwidth]{figs_supp/figure_2_small.png}
\caption{More visualization of predictions on CMU-Mocap (UMPM) dataset. Ours constantly show plausible and accurate predictions of human motion, especially during long-term motion. Best viewed when zoomed in.}
\label{CMU_VIZ}
\end{figure*}

\section{More qualitative results}
As shown in additional visualizations on CMU-Mocap (UMPM) dataset of Fig.~\ref{CMU_VIZ}, our t2p model generates more plausible motion for diverse behaviors. 
Indeed, our model was able to learn the specific physical mechanism of not only common motion such as walking forward (sequence 3, from top to bottom) but also unique behaviors such as punching (sequence 1) and walking backward (sequence 2).
The competence of our model is more clearly exhibited at later timesteps.
At timestep later than 1.5s, predictions of previous works more frequently show agents traversing in parallel feet, or manifesting physically unstable postures.
On the other hand, our T2P model predicts physically natural pose sequences at these timesteps, depicting the effectiveness of our coarse-to-fine approach in making long-term predictions.
As for the JRDB-GMP 2s/5s dataset, previous methods often predict motion that causes collision with other agents.
Our method, on the other hand, effectively models agent interaction even in complex scenes and predicts plausible pose sequences as shown in Fig.~\ref{JRDB_VIZ}

\section{Detailed dataset specifications}
\subsection{Construction of JRDB-GMP dataset}
Here, we elaborate on the details of constructing JRDB-GMP dataset.
As explained in the main paper, we use SOTA method for monocular scale-aware 3D pose extraction~\cite{sun2022putting} and both 2D pose annotation and 3D bounding boxes.
Algorithm~\ref{JRDB_algorithm} outlines the overall process:

\begin{algorithm}
    \caption{JRDB-GMP construction algorithm}
    \label{JRDB_algorithm}
    \begin{algorithmic}
    % \State $i \gets 10$
    \For{$t = 1$, $t{+}{+}$, while $t < T$}
        \For{$i = 1$, $i{+}{+}$, while $i <= 6$}
            \State{Extract $P_{t,i}^{3D,X}$}
            \State $N \gets \text{number of detected persons in} P^{3D,X}$
            \For{$n = 1$, $n{+}{+}$, while $n <= N$}
                \If{$L2(p_{t,i,n}^{2D,X}, \phi_{closest}(p_{t,i,n}^{2D,X}))<\tau$}
                    \State $p_{t,i,n}^{3D,X} \gets \phi_{pose}(p_{t,i,n}^{3D,X}, p_{t,i,n}^{3D,Y})$ 
                    \State $p_{t,i,n}^{3D,X} \gets \phi_{center}(p_{t,i,n}^{3D,X}, b_{t,i,n}^{Y})$
                    \State $p_{t,i,n}^{3D,X} \gets \phi_{rotate}(p_{t,i,n}^{3D,X})$
                    \If{$p_{t,i}^{3D}$ is not registered}
                        \State $\Tilde{p}_{t,i,n}^{3D,X} \gets \text{register}(p_{t,i,n}^{3D,X})$
                        % \State $\Tilde{p}_{t,i,n}^{3D,X}$ \gets register($p_{t,i,n}^{3D,X}$)
                    \EndIf
                \EndIf 
            \EndFor
        \EndFor
    \EndFor
    \end{algorithmic}
\end{algorithm}

Where $p_{t,i,n}^{3D,X} \in P_{t,i}^{3D,X}$, $p_{t,i,n}^{2D,X} \in P_{t,i}^{2D,X}$ denotes extracted 3D pose and its corresponding 2D pose mapped to the camera coordinates.
Also, $p_{t,i,n}^{2D,Y} \in P_{t,i}^{2D,Y}$ and $b_{t,i,n}^{Y} \in B_{t,i}^Y$ denote 2D pose annotation and 3D bounding box annotations.
$P_y^{3D}$ denotes 2D pose annotation projected in 3D world coordinates to represent viable proposals.
$\tau$ denotes the 2D keypoint L2 distance threshold for detection filtering.
$\phi_{closest}, \phi_{pose}, \phi_{center}$, and $\phi_{rotate}$ denotes algorithmic operations elaborates as below.

\noindent{$\bm{\phi_{closest}}$}\quad
The extracted 3D poses inevitably contains noise in its samples, since they are extracted via an algorithm.
We use 2D annotations to filter these outliers.
Namely, if L2 distance between the annotation joints $p_{t,i,n}^{2D,X}$ and 2D-projected 3D pose is larger than $\tau$ in 2D camera coordinates, the detected pose $p_{t,i,n}^{3D,X}$ is not used.

\noindent{$\bm{\phi_{pose}}$}\quad
Even after filtering the outliers, the dataset still contains some noise that influences the extracted 3D poses.
Therefore, we use 2D pose annotations to minimize these temporal jitters.
First, for each 2D pose of extracted 3D pose $p_{t,i,n}^{2D,X}$ of a person, we adjust the average x-axis value of its corresponding 2D annotation match $P_{t,i}^{2D,Y}$ to that of $p_{t,i,n}^{2D,X}$.
In doing so, the subsequent process only refines the only the local pose while its global position remains stationary.
The joint 3D position of an initially extracted 3D pose and its corresponding 2D camera coordinates of 2D pose annotation are given as $(x,y,z)$ and $(X,Y)$.
Then, a 3D line is drawn from $(0,0,z)$ to the 3D-projection of $(X,Y)$, namely $inv(K)\cdot (X,Y,1)$.
This line represents the possible 3D coordinates of the joint, given a 2D annotation.
The initially acquired 3D positions of the joint $(x,y,z)$ are adjusted to its closest point to the previously drawn line.
Such modification on each joint position corroborates the local accuracy of acquired 3D pose by minimizing the remnant noise via use of 2D pose annotation.

\noindent{$\bm{\phi_{center}}$}\quad
The aforementioned process $\bm{\phi_{pose}}$ only adjusts local motion, requiring an additional step for adjusting its global position.
For this purpose, the global $x,y$ positions of $p_{t,i,n}^{2D,X}$ is adjusted into the central $x_b,y_b$ positions of 3D bounding box annotation $b_{t,i,n}^Y$ of its match.
This refinement puts the detected 3D joints in their accurate global position.

\noindent{$\bm{\phi_{rotate}}$}\quad
3D poses are acquired for each view of omnidirectional 5 cameras of the robot.
Therefore, The acquired 3D poses of each view is rotated along the Z-axis to the front view, where Z-axis is where the robot is located.
In doing so, the 3D poses of all visible agents in 360$^{\circ}$ of a given scene are accurately acquired in global coordinates.

2D pose annotation $P_{t,i}^{2D,Y}$ and 3D bounding box annotations $B_{t,i}^Y$ both include agent numbers, which we use to temporally track the acquired 3D poses.
These agent IDs are used to register the refined pose to acquire the final 3D pose sequence $\Tilde{p}_{t,i,n}^{3D,X}\in \Tilde{P}^{3D,X}$.
Only the agents within 4.5 meters from the robot are considered, as agents beyond this threshold contains more noise than closer agents.
Also, we only consider sequences where at least 3 agents are present within 4.5 meters from the robot during the sequence of given scene.
In order to ensure a sufficient amount of training data that prevents underfitting, we parse the 1s/2s dataset by every 15 frames, and 2s/5s by every 3 frames.

\begin{figure*}[t]
\includegraphics[width=\textwidth]{figs_supp/figure_1_small.png}
\caption{Input images and 2D annotations (left column) used for extracting 3D poses (right column) on various indoor/outdoor scenes.}
\label{JRDB_dataset_viz}
\end{figure*}

\subsection{Visualization of JRDB-GMP dataset}
Figure~\ref{JRDB_dataset_viz} visualizes example scenes from the JRDB dataset along with its extracted poses. 
JRDB scenes include both indoor and outdoor scenes, both of which include scenes with various number of agents as less and two and as many as 25.
As depicted in the figure, 2D pose annotations are available for agents with slight occlusion, which we use to refine the extracted 3D pose.
Agents with severe occlusion are not detected by the monocular 3D pose extraction algorithm~\cite{sun2022putting}.
As a result, the JRDB-GMP dataset contains real world sequences of 3D poses with minimal amount of noise, depicting a long-term multi-agent environment.

\subsection{Limitation of JRDB-GMP dataset}
Since JRDB dataset is collected in a monocular setting, JRDB-GMP inevitably incorporates noise due to a lack of geometric constraints when regressing the 3D poses.
We have minimized these artifacts by refining the extracted 3D poses via 2D and 3D annotations as explained in the supplementary materials.
Their GIF examples of supplementary materials demonstrate the resulting natural sequences.
Despite such a pruning process, minimal noise remains with partially occluded bodies.
Pose annotation was often not available for these occluded parts, limiting their refinement process.
Nevertheless, our use of SoTA 3D pose extraction algorithm~\cite{sun2022putting} and subsequent maximal refinement has constructed a reliable testbed for human motion forecasting at the current technology level.
Certainly, we believe our acquisition strategy is well-suited and scalable in real-world scenes where IMU sensors are not available.

\section{Elaboration on dataset scenes}
JRDB dataset is comprised of 17 indoor (cafe, library, study room, etc) and 10 outdoor scenes (road, plaza, etc).
% It includes 26 actions as scrutinized in JRDB-Act~[CVPR 2022].
JRDB-Act~\cite{ehsanpour2022jrdb} scrutinizes the types and distribution of 26 actions included in the dataset.
% The dataset includes ~~action which is described in JRDB-Act~
Its most common actions are standing, walking, sitting, and holding sth. 
In addition, specific actions like cycling, going upstairs, eating, skating, and greeting gestures are also included by a non-trivial amount.
JRDB-GMP convers such varied representations of real-world behaviors.
3DPW is also collected in a real-world in-the-wild environment and includes diverse motions of two agents: dancing, riding bus, fencing, etc.
% CMU-Mocap (UMPM)~[\textcolor{mainPaperColor}{13},\textcolor{mainPaperColor}{62}] dataset blends two datasets to synthesize contrast of interaction.
% It includes 140$+$ category of sequences, diversely ranging from walking, running to dancing, throwing.
CMU-Mocap (UMPM) dataset includes 140+ categories of motion: rolling, dancing, throwing, and more.

In terms of geological features, the venues in JRDB-GMP and 3DPW incorporate diverse geometrical constraints.
Multi-agent interactions in such unique environments guide agents to traverse in diverse patterns.
For example, desks and rails in cafe and library compose convoluted scenes that naturally guide disparate non-linear trajectories.
% Coupled with behavior intention constraints, agents traverse in diverse linear and non-linear trajectories.
% 그냥 다양하다고 하면, ...
% Coupled with agent-specific behavioral constraints, agents traverse in diverse linear and non-linear trajectories.
CMU-Mocap (UMPM) also consists of varied locomotion modes since constructed to capture as diverse motion categories as possible.
Therefore, the datasets account for diverse trajectories that incorporate real-world environments.
Indeed, the trajectory-level human motion is already complex in a multi-agent environment, which is further convoluted by each local motion.
Our coarse-to-fine approach competently handles such complex task.

\begin{figure*}[h]
\includegraphics[width=\textwidth]{figs_supp/figure_3_small.png}
\caption{More visualization of predictions on JRDB-GMP 2s/5s. Unlike previous methods, our model predicts plausible future motion without collision with other agents. Best viewed when zoomed in.}
\label{JRDB_VIZ}
\end{figure*}

\section{Metrics}
Out of $F$ modes of prediction $\textbf{Y}$, the mode with minimum JPE metric is selected as the mode to calculate all metrics.\\
\textbf{APE}: Aligned mean per joint Position Error is used as a metric to evaluate the forecasted local motion.
$L2$ distance of each joint in the hip joint coordinate is averaged over all joints for a given timestep.\\
\begin{equation}
\begin{aligned}
\textup{APE($Po_{\mathcal{F}},\widehat{Po}_{\mathcal{F}})=\frac{1}{N\times J}\sum^N_{i=1}\sum^J_{j=1}\parallel Po_{\mathcal{F}_{j^i}} - \widehat{Po}_{\mathcal{F}_{j^i}} \parallel^2$}
\end{aligned}
\end{equation}
\textbf{FDE}: Final Distance Error evaluates the forecasted global trajectory by calculating the hip joint $L2$ distance of a given timestep. \\
\begin{equation}
\begin{aligned}
\textup{FDE($Tr_{\mathcal{F}},\widehat{Tr}_{\mathcal{F}})=\frac{1}{N}\sum^N_{i=1}\parallel Tr_{\mathcal{F}}^i - \widehat{Tr}_{\mathcal{F}}^i \parallel^2$}
\end{aligned}
\end{equation}
\textbf{JPE}: Joint Precision Error evaluates both global and local predictions by mean $L2$ distance of all joints for a timestep.
\begin{equation}
\begin{aligned}
\textup{JPE($\textbf{Y},\hat{\textbf{Y}})=\frac{1}{N\times J}\sum^N_{i=1}\sum^J_{j=1}\parallel \textbf{Y}_j^i - \hat{\textbf{Y}}_j^i \parallel^2$}
\end{aligned}
\end{equation}

Where N is the number of agents and J is the number of joints.

\section{Model architecture}
The model implemented with pytorch-lightning will be released publicly upon acceptance. 
We provide detailed description of the model as below:

\subsection{Pose encoder}
For DCT and MPBPConv layer, we adopt the same layer structure from TBIFormer~\cite{peng2023trajectory} with final feature dimension of 128.
Multi-head self-attention layer has 8 attention heads and input dimension of 128, with key/value/query dimension of 64.
After the multi-head attention layer, feature is expanded to 128 with mlp and passes a dropout layer of dropout rate 0.2.
The following FFN layer is composed of 2 linear layers of 128-1024-128, along with layer normalization with $\epsilon=1e-6$, drop out layer of 0.2, and skip connection.
The MSA and FFN layers are repeated $L=2$ times. 

\subsection{Trajectory module}
The trajectory module is composed of \textit{aaencoder} from HiVT~\cite{zhou2022hivt}.
This module is composed of a message passing module which computes agent-wise interaction in a trans-rotation invariant manner at each time step.
After passing the trajectory module, a feature is comprised of a latent with dimension 96 at each time step.

\subsection{Traj-pose module}
The pose embedding $Z_{Po}$ of dimension 128 is reduced to dimension 96 with a single linear layer.
Then, graph attention following Eq. 4 of the main manuscript is performed at every time step to get traj-pose embedding $Z$ of dimension 96.

\subsection{Trajectory decoder}
Trajectory decoder is composed of temporal encoder, aggregator, and a MLP layer.
The temporal encoder utilizes an extra learnable token of dimension 96 and temporal masks similar to BERT~\cite{devlin2018bert}.
There are sequentially 4 transformer encoder layer in the temporal encoder.
The aggregator is composed of a single message passing layer.
During message passing, its node is 96-dimsensional traj-pose embedding, and its edge is a 96-dimensional edge feature which is the output of a single mlp layer that takes the concatenation of edge attributes such as relative position and relative rotation angle.
The MLP layer is composed of two linear layers that gradually reduce the dimension to 192-96-future\_timestep$\times$3.
After first two linear layers, layer normalization and ReLU activation layers are followed.

\subsection{Pose decoder}
128-dimensional pose query is repeated num\_mode times, and concatenated with 96-dimensional traj query.
Then, a mlp layer reduces the concatenated query into 128 dimension.
The decoder is composed of 2 layers of multi-head attention decoder layers and 3 fully connected linear layers.
The multi-head attention decoder layers have the same structure as the multi-head attention encoder layers.
After three fully connected linear layers, inverse DCT is performed to recover the output to the location.

\section{Implementation details}
For our T2P model, 2 layers of pose encoder transformer are stacked, followed by 2 layers of transformer in pose decoder.
Embedding dimensions of 96 and 128 are used for trajectory and pose embeddings, respectively.
The transformed key, value dimension of 64 is used for all transformer architectures.
A learning rate of 0.003 is used with an AdamW optimizer with weight decay.
We train our model on a single NVIDIA A6000 GPU. 
Further details are included in the released code.

\section{More ablation study}
\subsection{Module ablation on CMU-Mocap (UMPM) dataset}
We report further ablation of module components on CMU-Mocap (UMPM) dataset.
Table.~\ref{tab:ablation_components_CMU} reports the influence of core components of our trajectory encoder and pose decoder on CMU-Mocap (UMPM) dataset.
We assess the significance of incorporating local pose embedding and modeling agent interaction in the trajectory encoder. 
Comparing experiments 1, 5, and 3, 4, all demonstrate enhancements in JPE and FDE metrics when utilizing local pose embedding. 
Our approach leverages detailed local pose cues to deduce an agent's global intention, with a more pronounced improvement in JPE and FDE observed when considering agent interaction (exp. 1, 5). 
Indeed, factoring in the interaction between local motion cues amplifies the advantages of predicting global motion intents for all agents.
Regarding interaction modeling, its application proves advantageous for both global and local forecasts, as evident in experiments 4 and 6. 
These collective enhancements underscore the importance of accounting for local and global motion interactions in their respective forecasts.
Turning to the pose decoder, comparisons between experiments 2, 4 and 5, 6 reveal consistent improvements in the APE metric. 
This consistent enhancement validates the efficacy of the trajectory-conditioned local motion forecast approach in generating plausible local motion from global intention.

\begin{table}[h]
\caption{Ablation studies on core components of model structures. Experiments are done with CMU-Mocap (UMPM) dataset with 1s as given and 2s of forecasted horizon.}
\vspace{-5pt}
\label{tab:ablation_components_CMU}
\resizebox{\linewidth}{!}{
\begin{tabular}{c|ccc|ccc}
\toprule
\multirow{2}{*}{\begin{tabular}[c]{@{}c@{}}Exp. \\ \#\end{tabular}} & \multicolumn{2}{c|}{Trajectory encoder}                                                                                                                         & Pose decoder                                                        & \multicolumn{3}{c|}{Metrics}                                                                  \\ \cline{2-7} 
                        & \multicolumn{1}{c|}{\begin{tabular}[c]{@{}c@{}} Local pose \\ embedding\end{tabular}} & \multicolumn{1}{c|}{\begin{tabular}[c]{@{}c@{}}Agent \\ interaction\end{tabular}} & \begin{tabular}[c]{@{}c@{}} Trajectory\\ -conditioning\end{tabular} & \multicolumn{1}{c|}{\begin{tabular}[c]{@{}c@{}}JPE \\ @5s\end{tabular}} & \multicolumn{1}{c|}{\begin{tabular}[c]{@{}c@{}}APE \\ @5s\end{tabular}} & \multicolumn{1}{c|}{\begin{tabular}[c]{@{}c@{}}FDE \\ @5s\end{tabular}} \\ \hline
-                       &                                                                                     &                                                                                      &                                                                       & 290.9                         & 160.8                         & 228.5                         \\ 
1                       &                                                                                     & \checkmark                                                                                    &                                                                       & 270.7                         & 153.9                          & 197.6                         \\ 
2                       & \checkmark                                                                                   &                                                                                      &                                                                       & 275.2                         & 154.9                          & 200.8                         \\ 
3                       &                                                                                     &                                                                                      & \checkmark                                                                     & 273.8                        & 153.2                          & 201.5                         \\
4                       & \checkmark                                                                                   &                                                                                      & \checkmark                                                                     & 272.9                         & 152.4                          & 200.8                         \\ 
5                       & \checkmark                                                                                   & \checkmark                                                                                    &                                                                       & 268.7                         & 153.9                          & 193.7                         \\ 
6                       & \checkmark                                                                                   & \checkmark                                                                                    & \checkmark                                                                     & \textbf{262.7}                         & \textbf{151.7}                          & \textbf{188.9}                         \\ \bottomrule
\end{tabular}%
}
\vspace{-5pt}
\end{table}

\subsection{Forecast on fine-grained motion}
Our model also shows competence on fine-grained motion, which we characterize as action with minimal global displacement.
Indeed, global and local intentions contain complementary hints even for fine-grained motion.
For example, let's consider two stationary people shaking hands.
Their stationary and adjacent trajectories capture the presence of coarse interaction.
Then, their detailed local motion of shaking hands or greeting corroborates the modeled interaction.
When generating forecasts, initial immobile trajectories represent the encoded static interaction.
Fine-grained motion such as hand-shaking is then conditionally predicted from such coarse intention of stationary trajectories.
% As the coarse intention is exploited to infer fine-grained motion and vice versa, a single branch would suffice for each mode.
% Specifically, coarse trajectory connotes the coarse intention of interaction and motion, and its collective modeling along with local motion 
Table~\ref{fine_grained} shows prediction results for fine-grained motion, CMU-Mocap (UMPM) dataset samples thresholded by trajectory displacement of past motion.
Our method is superior for all metrics; specifically, optimal performance in APE metric highlights our competence in capturing and forecasting the fine-grained local motion.
Qualitatively, for the top row red person of Fig. 1 in supplementary materials, ours' predicts a more dynamic punching motion for the stationary agent.

\begin{table}[h]
\centering
\vspace{-6.5pt}
\caption{Comparison of performance on fine-grained motion on CMU-Mocap (UMPM) dataset.}
\label{fine_grained}
\vspace{-6.5pt}
\resizebox{\columnwidth}{!}{%
\begin{tabular}{|c|ccc|ccc|}
\hline
\multicolumn{1}{c|}{\begin{tabular}[c]{@{}c@{}} Global displacement \\ threshold (m)\end{tabular}} & \multicolumn{3}{c|}{$<$0.05}                                                               & \multicolumn{3}{c|}{$<$0.2}                                                                  \\ \hline
Metric @ 2s & \multicolumn{1}{c|}{APE}           & \multicolumn{1}{c|}{JPE}           & FDE           & \multicolumn{1}{c|}{APE}            & \multicolumn{1}{c|}{JPE}            & FDE           \\ \hline
MRT~\cite{wang2021multi}         & \multicolumn{1}{c|}{108.7}         & \multicolumn{1}{c|}{140.8}         & 71.8          & \multicolumn{1}{c|}{138.1}          & \multicolumn{1}{c|}{180.6}          & 99.0          \\ \hline
JRT~\cite{xu2023joint}         & \multicolumn{1}{c|}{92.9}          & \multicolumn{1}{c|}{104.6}         & 44.8          & \multicolumn{1}{c|}{129.7}          & \multicolumn{1}{c|}{157.8}          & 94.9          \\ \hline
TBIFormer~\cite{peng2023trajectory}   & \multicolumn{1}{c|}{93.2}          & \multicolumn{1}{c|}{156.9}         & 105.8         & \multicolumn{1}{c|}{127.8}          & \multicolumn{1}{c|}{189.6}          & 128.1         \\ \hline
Ours        & \multicolumn{1}{c|}{\textbf{87.6}} & \multicolumn{1}{c|}{\textbf{93.1}} & \textbf{22.6} & \multicolumn{1}{c|}{\textbf{122.9}} & \multicolumn{1}{c|}{\textbf{146.3}} & \textbf{65.1} \\ \hline
\end{tabular}%
}
\vspace{-12pt}
\end{table}

\setlength{\columnsep}{7pt}
\begin{wrapfigure}{r}[-15pt]{0.075\textwidth}
\vspace{-15pt}
% \setlength{\columnsep}{-1.3in}%
% \hspace{-.30in}
  \centering
    \includegraphics[width=0.111\textwidth]{figs_rebut/rebuttal_fig_1.png}  
\vspace{-11.5pt}
% \hspace{-.30in}
\caption{\mbox{Unnatural motion} \mbox{GT data example.}}
\label{unnatural_motion}
\vspace{-10pt}
\end{wrapfigure}

\section{Failure cases}
Our method, along with previous works, failed when local and global motion did not share consistent intentions.
One example could be found in the CMU-Mocap (UMPM) dataset.
As it was constructed with diversity as a priority, a few random motions such as flapping arms while walking could be found as in Fig.~\ref{unnatural_motion}.
Such a sequence lacks consistency between the local motion of flapping and the global motion of walking.
As the intentions are misaligned, complementary contributions towards each decoding were marginal.
% As the intentions are misaligned, complementary contributions towards each decoding were marginal and resulted in a poor forecast.
Aside from these outliers, our method improved on sequences comprised of natural motion for all datasets.
